# Supplementary material for: Learning Patient-Specific Disease Dynamics with Latent Flow Matching for Longitudinal Imaging Generation
Source: arXiv:2512.09185 source file (2026-06-17)
Supplement: Supplementary file 1 [file X_suppl.tex]

\clearpage

\appendix
\section{Appendix}

Similar to Litrici \etal~\citep{litrico2024tadm}, we encode the given query time $t$ and the futuer time $t+\Delta t$ via a positional time embedding sinusoidal positional encoding. In our design, we use Vision Transformer (ViT) architecture for Diffusion denoiser and the ControlNet.

\subsection{ArcRank: Longitudinal Contrastive Alignment of Anatomy}
\label{sec:arcrank}
In longitudinal data, each subject’s scans form a trajectory of change.  
We wanna enforce the learning of patient-specific disease progression trcjectory in latent space. Most contrastive loss in afore-mentioned caseds pull similar image together, ie put same imaging from same patient together interchangeably close, without indicating which is earlier., or pulls adjacent timepoints together, but we might also want to encode directionality (i.e. understanding that one comes before the other linewise), to better sample it when inference new future latent.
The latent mitigates the risk that the generative model produces a future scan resembling a different patient. 

Inspired by ArcFace Loss, that propose to pull the angle from same group similar. We propose \ourfeature, which consistitude two parts, the firts align different timepoint along with the same angle line, effectively learning an identity vector that captures stable person-specific attribute. The second to make it chronicolly meaning, we propose the ranking part that is pull，  time-aware loss further arranges the latent space so that time progression is encoded smoothly， scans that are close timepoint, end up close in representation，  whereas scans longer apart diverge.

This is conceptually similar to Longitudinal Neighborhood Embedding (LNE) approaches~\citep{ouyang2022self}
propose a smooth trajectory field where each trajectory captures changes in brain ages between a pair of MRIs extracted from a longitudinal sequence. Our method is also learn a vector field that in each patient aligns with same angle (direction), but the magnitude is varies according to the state， modulate its output based on “how far along” the patient’s trajectory is, leading to more accurate progression trends.

A patient with temporally ordered image features $\mathbf{f}_i,\mathbf{f}_j$ at times $t_i < t_j$, we define the ArcRank loss by combining an angular alignment term with a norm-ranking term:

\begin{equation}
\mathcal{L}_{\text{ArcRank}} = \sum_{\substack{i<j\\ \text{same patient}}}
\left[ \angle(\mathbf{f}_i, \mathbf{f}_j) + \lambda\, \max\left(0,\,\|\mathbf{f}_i\| + m - \|\mathbf{f}_j\|\right) \right],
\end{equation}

where
\begin{equation}
\angle(\mathbf{f}_i, \mathbf{f}_j) = \arccos\left(\frac{\mathbf{f}_i \cdot \mathbf{f}_j}{\|\mathbf{f}_i\| \|\mathbf{f}_j\|}\right)
\end{equation}
is the angular (geodesic) distance between feature vectors. Here, $\lambda > 0$ balances the two terms, and $m > 0$ is a margin that enforces strict norm ordering.

\paragraph{Angular Term:} The angle term $\angle(\mathbf{f}_i, \mathbf{f}_j)$ encourages same-patient features to align directionally on the unit hypersphere. This is analogous to contrastive self-supervised learning approaches that optimize cosine similarity. See: 

On the Importance of Embedding Norms in Self-Supervised Learning, and angular-margin methods like  AMC-Loss.

\paragraph{Rank Term:} The hinge loss $\max(0, \|\mathbf{f}_i\| + m - \|\mathbf{f}_j\|)$ ensures that feature norms increase with time: later-time features must have strictly greater norm than earlier ones. This leverages the fact that embedding norm magnitudes often correlate with semantic richness or confidence.

% Magnitude Ranking Across Timepoints, 
\begin{itemize}
    \item $\lambda$: trade-off between angular and chronological alignment.
    \item $m$: margin to ensure meaningful norm separation.
\end{itemize}

Minimizing $\mathcal{L}_{\text{ArcRank}}$ aligns same-patient features angularly while enforcing temporal ordering through vector norm ranking. The loss is fully self-supervised, relying only on patient identity and the intrinsic order of timestamps.

\paragraph{Scaling Function Term:} 
$$
\mathbf{f}_{t+\Delta t} = \gamma_t \cdot \mathbf{f}_t
$$

Where $\gamma\_t$ is a scalar field (same spatial shape as $\mathbf{f}\_t$), predicting how much to scale the magnitude at each point.

Then, train a network to predict $\gamma\_t$ given:

 $\mathbf{f}\_t$
 optionally, an image or anatomical context at $t$ or $t+\Delta t$

 Loss Function to Supervise $\gamma\_t$

If you have ground truth $\mathbf{f}\_{t+\Delta t}$, then supervise:

$$
\mathcal{L}_{\text{scale}} = \left\| \gamma_t \cdot \mathbf{f}_t - \mathbf{f}_{t+\Delta t} \right\|^2
$$

If only magnitudes are known:

$$
\mathcal{L}_{\text{mag}} = \left\| \gamma_t \cdot \|\mathbf{f}_t\| - \|\mathbf{f}_{t+\Delta t}\| \right\|^2
$$

   % In effect, this tackles the problem of patient heterogeneity: two patients with different baseline embeddings will produce different future outcomes, aligning with individualized disease paths rather than an average trajectory.

% Controllable Consistency in Image or Video
% Generation via Reference Feature Guidance

\subsection{Preliminary: Latent Flow Matching}
Flow Matching (FM)~\citep{lipman2023flow} learns a continuous transport map between two distributions over a data space $\mathcal{X} \subseteq \mathbb{R}^d$, using only samples and without access to likelihoods.
Latent Flow Matching (LFM)~\citep{dao2023flow,chadebec2025lbm} extends FM by introducing a lower-dimensional latent space $\mathcal{Z}$. An encoder $E_\phi: \mathcal{X} \to \mathcal{Z}$ maps data into this latent space, where a transport map is learned, \ie $\mathbf  z := E_\phi(\mathbf x)$.

Let $\pi_0, \pi_1$ be distributions over the latent space $\mathcal{Z} \subseteq \mathbb{R}^d$. Define a time-dependent velocity field $v : \mathcal{Z} \times [0,1] \to \mathbb{R}^d$ and consider a stochastic process $(\mathbf{z}_t)_{t \in [0,1]}$ governed by the stochastic differential equation (SDE):
\begin{equation}\label{eq:sde}
\mathrm{d}\mathbf{z}_t = v(\mathbf{z}_t, t)\mathrm{d}t + \sigma(\mathbf{z}_t, t)\mathrm{d}B_t, \quad \mathbf{z}_0 \sim \pi_0,
\end{equation}
where $B_t$ is standard Brownian motion and $\sigma$ is the diffusion coefficient. In practice, $v$ is approximated using the analytically defined target velocity field:
\begin{equation}
v^*(\mathbf{z}_t, t) := \frac{\mathbf{z}_1 - \mathbf{z}_t}{1 - t}, \quad (\mathbf{z}_0, \mathbf{z}_1) \sim \pi_0 \times \pi_1,
\end{equation}
with intermediate states $\mathbf{z}_t$ sampled from the stochastic interpolant (deterministic when $\sigma \to 0$):
\begin{equation}\label{eq:interpolant}
\mathbf{z}_t = (1 - t)\mathbf{z}_0 + t\mathbf{z}_1 + \sigma \sqrt{t(1 - t)}\epsilon, \quad \epsilon \sim \mathcal{N}(0, I).
\end{equation}

A neural velocity field $v_\theta(\mathbf{z}, t)$ is trained to match $v^*$ by minimizing the following error:
\begin{equation}\label{eq:fm_loss}
\mathcal{L}_{\mathrm{LFM}}(\theta) = \mathbb{E}_{t, \mathbf{z}_0, \mathbf{z}_1, \epsilon} \left[\left| v_\theta(\mathbf{z}_t, t) - \frac{\mathbf{z}_1 - \mathbf{z}_t}{1 - t} \right|^2\right].
\end{equation}

Once trained, the learned velocity field $v_\theta$ is used to integrate the SDE in Eq.~\eqref{eq:sde}, transporting samples from $\mathbf{z}_0$ toward $\mathbf{z}_1$. The final outputs in the original data space are obtained by decoding the transported latent samples: $\mathbf x_1 := D_\psi(\mathbf{z}_1)$.

% -------

Let $\pi_0$ and $\pi_1$ be two distributions over a data space $\mathcal{X} \subseteq \mathbb{R}^d$, Flow Matching~\citep{lipman2023flow} aims to learn a continuous transformation that transports $\pi_0$ to $\pi_1$ using only samples from $\pi_0$, without requiring explicit likelihoods.

Flow Matching defines a time-dependent velocity field $v : \mathcal{X} \times [0,1] \to \mathbb{R}^d$, or optimal transport (OT), and models a stochastic process $(x_t)_{t \in [0,1]}$ via the SDE:
\begin{equation}\label{eq:sde}
dx_t = v(x_t, t),dt + \sigma(x_t, t),dB_t, \quad x_0 \sim \pi_0,
\end{equation}
where $B_t$ is Brownian motion and $\sigma$ is the diffusion coefficient.  In practice, the velocity is typically defined in the analytic field: $v^*(x_t, t) := (x_1 - x_t)/ (1 - t)$ based on sample pairs $(x_0, x_1) \sim \pi_0 \times \pi_1$. A corresponding stochastic interpolant is then constructed as:
\begin{equation}\label{eq:interpolant}
x_t = (1 - t)x_0 + t x_1 + \sigma \sqrt{t(1 - t)}\epsilon,\quad \epsilon \sim \mathcal{N}(0, I),
\end{equation}
defining a stochastic transport mapping between $x_0$ and $x_1$ (deterministic when $\sigma \to 0$).

When training, a Markovian approximation is learned by regressing a neural network $v_\theta(x_t, t)$ to the ideal velocity field $v^*$ via the following loss:
\begin{equation}\label{eq:fm_loss}
    \mathcal{L}_{\mathrm{FM}}(\theta) = \mathbb{E}_{t, x_0, x_1, \epsilon} \left[\left\| (x_1 - x_t)/(1 - t) - v_\theta(x_t, t) \right\|^2\right].
\end{equation}

Finally, the estimated drift function $v_{\theta}$ can be integrated into standard SDE solvers to solve Eq.~\eqref{eq:sde} to generate samples that follow $\pi_1$ from initial samples drawn from $\pi_0$.

Latent Flow Matching (LFM)~\citep{dao2023flow,chadebec2025lbm} extends this framework to high-dimensional data by introducing a latent space $\mathcal{Z}$ and mapping the data into it via an encoder $E_\phi: \mathcal{X} \to \mathcal{Z}$. In the latent space, a flow field $v_\theta(\mathbf{z}, t)$ is learned to match the interpolated distributions between $E_\phi(\pi_0)$ and $E_\phi(\pi_1)$. This shift enables efficient modeling of complex data distributions, leveraging lower-dimensional latent representations where flows are more tractable.

The training objective in LFM typically involves matching the flow field to samples from an analytically defined reference process, such as a displacement interpolation (\eg~linear or optimal transport paths) between latent encodings. A decoder $D_\psi: \mathcal{Z} \to \mathcal{X}$ is then used to map latent trajectories back to data space, allowing sample generation and density estimation through integration of the learned ODE in latent space followed by decoding.

% -----------------------
\subsection{AnaGraph: Representing Masks as Graph Nodes}
\label{sec:anagraph}

We propose AnaGraph, a graph-based representation that models anatomical structures in medical images. Each node corresponds to a segmented region, forming a graph that captures spatial relationships at baseline. The goal, however, is to predict anatomy at a future time point. A static graph provides limited information about how anatomy evolves. To address this, we introduce a morph function $M(\cdot)$ that deforms the baseline graph toward the future anatomy. This warped baseline segmentation acts as a proxy for future anatomy, offering directional cues to enable temporally informed predictions.

Given an image $x$ with its corresponding segmentation map $s$, we construct a graph representation $G = (\mathcal V, \mathcal E)$, where $V = \{ v_i \}_{i=1}^{N}$ denotes the set of $N$ segmented regions, $E = \{ e_{ij} \mid d(v_i, v_j) \leq \tau \}$ represents the edges based on spatial proximity $d(v_i, v_j)$ with a distance threshold $\tau$. We denote the graph construction process as $\mathcal{G}=G(x, s, a)$ from $x$ and patients attributes from notes $a$. These features can be viewed as a set of unordered nodes which are denoted as $\mathcal{V}=\{v_1,v_2,\cdots,v_N\}$.  We employ the Vision Graph (ViG)~\citep{han2022vision} to propagate information across segmented regions and encode their relationships within a latent space.

% the diffusion model and 

We aim to predict future anatomical segmentations using a graph-based model supervised by Dice loss. At time $t$, we initialise an anatomical graph $\mathbf{g}_t$ with node features from segmentation masks $\{s_{t,1}, s_{t,2}, \dots, s_{t,n}\} \sim \mathcal{S}$.

To model temporal change, we apply a morph function $M(\cdot)$ implemented via a Vision Graph (ViG)~\citep{}, which follows a ViT-style encoder-decoder. The predicted future mask $M(\mathbf{g}_t)$ is trained against the ground truth $s_{t+\Delta t}$ using:

\begin{equation}
\mathcal{L}_{\text{dice}} = 1 - \text{Dice}(M(\mathbf{g}_t), \mathbf{g}_{t+\Delta t})
\end{equation}
The goal is to learn meaningful  embeddings that preserve the biological geometric structure  while encoding region-wise interactions. This learned middle representation is then used as a conditioning feature for the diffusion model.

\paragraph{\ourgraph~guided Control Process}
After pretraining \ourgraph, we integrate it into the ControlNet framework. Specifically, we use the encoder $M_{\small E}$ to extract anatomical features, which are injected into each layer of ControlNet as conditional input. The encoder remains trainable to adapt its representations to the control task.

% The above graph-level processing can be denoted as $X'=\text{GraphConv}(X)$. 

\section{Rationale}
\label{sec:rationale}
Having the supplementary compiled together with the main paper means that:
\begin{itemize}
\item The supplementary can back-reference sections of the main paper, for example, we can refer to \cref{sec:intro};
\item The main paper can forward reference sub-sections within the supplementary explicitly (e.g. referring to a particular experiment); 
\item When submitted to arXiv, the supplementary will already included at the end of the paper.
\end{itemize}
To split the supplementary pages from the main paper, you can use \href{https://support.apple.com/en-ca/guide/preview/prvw11793/mac#:~:text=Delete%20a%20page%20from%20a,or%20choose%20Edit%20%3E%20Delete).}{Preview (on macOS)}, \href{https://www.adobe.com/acrobat/how-to/delete-pages-from-pdf.html#:~:text=Choose%20%E2%80%9CTools%E2%80%9D%20%3E%20%E2%80%9COrganize,or%20pages%20from%20the%20file.}{Adobe Acrobat} (on all OSs), as well as \href{https://superuser.com/questions/517986/is-it-possible-to-delete-some-pages-of-a-pdf-document}{command line tools}.
